# Supplementary material for: The Role of Partisan Culture in Mental Health Language Online
Source: arXiv:2506.20377 source file (2025-06-25)
Supplement: Supplementary file 1 [file Partisan_Culture_Supplementary_Information.pdf]

The Role of Partisan Culture in Mental Health Language Online
Supplementary Material
Supplement A
Mental Health Subreddits

7cupsoftea
abuse
adhd
adhdmeme
adhdwomen
adultsurvivors
advice
afterthesilence
agoraphobia
anger
anxiety
aspergers
aspiememes
autism
backonyourfeet
bipolar
bipolarreddit
bipolarsos
bpd
breakups
bullying
calmhands
compulsiveskinpicking
confession
confessions
cptsd
depressed
depression
domesticviolence
dpdr
emotionalabuse
existential_crisis
foreveralone
getting_over_it
gfd
griefsupport
hardshipmates
helpmecope
heretohelp
itgetsbetter
lonely
lostalovedone
makenewfriendshere
maladaptivedreaming
mentalhealth
mmfb
needafriend
ocd
offmychest
panicparty
psychosis
psychoticreddit
ptsd
ptsdcombat
radical_mental_health
rant
rapecounseling
reasonstolive
schizophrenia
socialanxiety
stopselfharm
suicidebereavement
suicidewatch
survivorsofabuse
survivorsunited
therapy
traumatoolbox
trichsters
vent

The Role of Partisan Culture in Mental Health Language Online
Supplementary Material
Supplement B
Republican Partisan Subreddits

**Method: Subreddit Labeling**

Partisan culture encapsulates many aspects of partisanship, including shared ideological values, norms, worldviews, and electoral practices. For future researchers, the first two authors of the study labeled the following Republican subreddits as being primarily ideologically partisan (e.g. focused around a specific partisan ideology) or electorally partisan (e.g. focused around electoral choices). Both authors were fully aligned, resulting in a Cohen's kappa agreement of 1.00.

askthe_donald (electoral)
asktrumpsupporters (electoral)
ask_thedonald (electoral)
conservative (ideological)
conservatives (ideological)
donaldtrump (electoral)
donald_trump (electoral)
gunpolitics (ideological)
kasichforpresident (electoral)
marco_rubio (electoral)
metarepublican (ideological)
progun (ideological)
prolife (ideological)
randpaul (electoral)
republican (ideological)
republicans (ideological)
republicansforsanders (electoral)
romney (electoral)
tedcruzforpresident (electoral)
theleftcantmeme (ideological)
the_donald (electoral)
the_donald_ca (electoral)
trump (electoral)
trump16 (electoral)
vote_trump (electoral)
walkaway (ideological)

The Role of Partisan Culture in Mental Health Language Online
Supplementary Material
Supplement C
Democrat Partisan Subreddits

**Method: Subreddit Labeling**

Partisan culture encapsulates many aspects of partisanship, including shared ideological values, norms, worldviews, and electoral practices. For future researchers, the first two authors of the study labeled the following Democrat subreddits as being primarily ideologically partisan (e.g. focused around a specific partisan ideology) or electorally partisan (e.g. focused around electoral choices). The Cohen's kappa agreement of the two first authors was of .94, with disagreements around the grassrootsselect and bernieblindness subreddits. These disagreements were settled through discussion and another round of labeling till both labeling authors were in alignment.

alexandriaocasio (electoral)
anarchism (ideological)
aoc (electoral)
askaliberal (ideological)
askberniesupporters (electoral)
askdemocrats (electoral)
askhillarysupporters (electoral)
bernie (electoral)
bernieblindness (electoral)
berniesanders (electoral)
beto2020 (electoral)
bluemidterm2018 (electoral)
capitalismvsocialism (ideological)
capitolconsequences (ideological)
centrist (ideological)
dankleft (ideological)
democraticparty (electoral)
democrats (electoral)
democrats2020 (electoral)
elizabethwarren (electoral)
enlightenedcentrism (ideological)
enoughcommiespam (ideological)
enoughsandersspam (ideological)
enough_sanders_spam (ideological)
grassrootsselect (ideological)
gravelforpresident (electoral)
hillaryclinton (electoral)
hillaryforamerica (electoral)
inslee2020 (electoral)
joebiden (electoral)
justicedemocrats (electoral)
kamala (electoral)
kossacks_for_sanders (electoral)
latestagecapitalism (ideological)
leopardsatemyface (ideological)
lessig2016 (electoral)
liberal (ideological)
moderatepolitics (ideological)
murderedbyaoc (electoral)
neoliberal (ideological)
obama (electoral)
ourpresident (electoral)
parlerwatch (ideological)
pete_buttigieg (electoral)
politicaldiscussion (ideological)
politicalhumor (ideological)
political_revolution (electoral)
politics (ideological)
presidentwarren (electoral)
progressive (ideological)
reform_the_dnc (ideological)
sandersforpresident (electoral)
shitliberalssay (ideological)
shitpoliticssays (ideological)
shitstatistssay (ideological)
socialism (ideological)

socialistra (ideological)
stillsandersforpres (electoral)
stupidpol (ideological)
thanksobama (ideological)
timcanova (electoral)
tulsi (electoral)
voteblue (electoral)
wayofthealoha (electoral)
wayofthebern (electoral)
yangforpresident (electoral)
yangforpresidenthq (electoral)
yanggang (electoral)

The Role of Partisan Culture in Mental Health Language Online
Supplementary Material
Supplement D
LIWC Categories

The Linguistic Inquiry and Word Count (LIWC) [13] text analysis tool organizes words into 74 categories that correspond with psycholinguistic attributes (such as language indicative of cognitive processing or of positive affect) or content themes (such as religious language or language related to bodily functions), and has been used in past CSCW and HCI research to find cultural differences in how people express distress [3, 12]. In our study, building on this past research, we conduct a similar analysis to understand where there might be differences between how Republican, Democrat, and unaffiliated users of online mental health support forums express distress.

We choose to highlight and center our analysis around 19 LIWC categories that past literature suggests might align with meaningful differences in expressions of distress between Republicans and Democrats. Below, we name those categories (in **bolded** text, with some example words listed) and describe the past literature that justified our choice of these categories, including literature from medical anthropology and psychology around cultural differences in expressions of distress, literature from political science on broad differences between Republicans and Democrats, and sociological literature on dimensions of increased polarization among Republicans and Democrats within non-political spaces in the United States.

**LIWC Dimensions of Analysis**

The **Social** (e.g. “talk”, “friend”) LIWC category: Past work has described the importance of social connections in how people seek support for their mental health [1] and how people come to understand and express their partisan identities [4]. We include the **Social** LIWC dimension to investigate whether there may be differences in the extent to which Republican and Democrat users discuss social connections (such as friends or family) as an aspect of their experiences of distress.

The **Male** (e.g. “dad”, “his”) and **Female** (e.g. “mom”, “her”) LIWC categories: Similar to our inclusion of the **Social** LIWC category, we also include the **Male** and **Female** LIWC categories to understand the kinds of social connections that Republican and Democrat users discuss in their expressions of distress, and whether there may be differences in terms of the level of gendered language that might be used. This is rooted in past research demonstrating that Republican politicians use more masculine-gendered language than Democrat politicians [15] — we include these dimensions to examine whether this dynamic may trickle down to how Republican and Democrat users of mental health support forum users express distress as well.

The **Cognitive Processing** (e.g. “know”, “think”, “because”) LIWC category: Past work has demonstrated that the **Cognitive Processing** language can be indicative of analytical thinking and reflective discussion of experiences [13]. We include this category to evaluate whether Republican and Democrat users of online mental health forums may be using the platforms in different ways — for example, to collectively

process experiences of distress (if cognitive processing language is higher) or to directly discuss their life events (if cognitive processing language is lower).

The **Positive Emotion** (e.g. “nice”, “sweet”) and **Negative Emotion** (e.g. “hurt”, “nasty”) LIWC categories: Following past research on cultural differences in expressions of distress in CSCW [3, 12], we include the Positive Emotion and Negative Emotion categories to understand the level to which Republican and Democrat users may be discussing feeling states in their support forum posts. We investigate whether there may be differences in the level of emotion openly discussed, as lower levels of open discussion of emotion may be indicative of the influence of stigma as in clinical mental health settings [5].

The **Anxiety** (e.g. “worried”, “fearful”) and **Anger** (e.g. “hate”, “annoyed”) LIWC categories: We include the **Anxiety** and **Anger** categories to understand whether specific sensory or emotional states are discussed to a greater extent among Republican and Democrat users in their expressions of distress. Differences between Republican and Democrat users may indicate partisan inclinations to frame distress in a given way (e.g. around anxiety or around anger), which could have implications for future help-seeking.

The **Feel** (e.g. “feels”, “touch”)**, Bio** (e.g. “blood”, “pain”), **Body** (e.g. “head”, “spit”), and **Health** (e.g. “flu”, “pill”) LIWC categories: Past research from medical anthropology [10], from CSCW [3, 12], and from HCI [11]  has demonstrated that minority populations (such as those of the Global South [11]) and populations with higher levels of stigma (such as those in rural areas of the U.S. [12]) can have high levels of somatic and physical language in their online expressions of distress. In line with this past work, we examine whether this pattern holds for Republican and Democrat users of mental health forums, acknowledging past research on intersections between stigma [9] and psychiatric language [6] in how partisans discuss their experiences of distress.

The **Affiliation** (e.g. “ally”, “friend”) LIWC category: Past research has described how an increase in partisan polarization has led to “us-versus-them” worldviews among Republican and Democrat partisans [7]. We include the **Affiliation** category to examine whether this “us-versus-them” social dynamic may be a part of the online expressions of distress from Republican and Democrat support forum users.

The **Work** (e.g. “job”, “majors”), **Leisure** (e.g. “cook”, “chat”), and **Home** (e.g. “kitchen”, “landlord”) LIWC categories:  Similar to our use of the **Social**, **Male**, and **Female** LIWC categories, we include these LIWC categories as dimensions of analysis to understand the kind of stressors that partisan individuals might discuss in their expressions of distress online, and whether there might be differences between how Republican and Democrat users utilize online mental health forums (for example, for collective processing versus direct reporting of daily life events).

The **Money** (e.g. “owe”, “cash”) LIWC category: Following past research in CSCW [12], we utilize the **Money** LIWC attribute to understand whether issues around income and class might be discussed by Republican and Democrat users. Past work in political science has described how class might be a uniting issue among polarized Republicans and Democrats [2] — the appearance of language around class in

online expressions of distress may indicate that economic stressors might be more acutely described online by one partisan group and be linked to how they conceptualize their distress.

The **Religion** (e.g. “altar”, “church”) LIWC category: Past work [16] has described the core role that religion plays in Republican partisan culture — we included this LIWC category as a dimension of analysis to investigate whether the religious aspects of Republican partisan culture also appear in Republican expressions of distress online.

The **Death** (e.g. “kill”, “bury”) LIWC category: Following past research in HCI [12], we utilize the **Death** LIWC category as one signal for the presence of language around suicide, particularly in light of the fact that rural areas (that tend to largely be Republican [14]) also have significantly higher rates of suicide [8].

**References**

[1] Lærke Mai Bonde Andersen, Amanda Nikolajew Rasmussen, Nicola J. Reavley, Henrik Bøggild, and Charlotte Overgaard. 2021. The social route to mental health: a systematic review and synthesis of theories linking social relationships to mental health to inform interventions. SSM-Mental Health 1, Article 100042, 15 pages.

[2] Clem Brooks and Jeff Manza. 1997. Social cleavages and political alignments: US presidential elections, 1960 to 1992. American Sociological Review 62, 6, 937-946.

[3] Munmun De Choudhury, Sanket S. Sharma, Tomaz Logar, Wouter Eekhout, and René Clausen Nielsen. 2017. Gender and cross-cultural differences in social media disclosures of mental illness. In Proceedings of the 2017 ACM Conference on Computer Supported Cooperative Work and Social Computing (CSCW '17), 353-369. https://doi.org/10.1145/2998181.2998250

[4] Steven Greene. 1999. Understanding party identification: A social identity approach. Political Psychology 20, 2, 393-403.

[5] Claire Henderson, Sara Evans-Lacko, and Graham Thornicroft. 2013. Mental illness stigma, help seeking, and public health programs. American Journal of Public Health 103, 5, 777-780.

[6] S. Y. Jesse and Nick Haslam. 2024. Broad concepts of mental disorder predict self-diagnosis. SSM-Mental Health, Article 100326, 8 pages.

[7] Nathan P. Kalmoe and Lilliana Mason. 2022. Radical American Partisanship: Mapping Violent Hostility, Its Causes, and the Consequences for Democracy. University of Chicago Press.

[8] Benson S. Ku, Jianheng Li, Cathy Lally, Michael T. Compton, and Benjamin G. Druss. 2021. Associations between mental health shortage areas and county-level suicide rates among adults aged 25 and older in the USA, 2010 to 2018. General Hospital Psychiatry 70, 44-50.

[9] Christin L. Munsch, Liberty Barnes, and Zachary D. Kline. 2020. Who's to blame? Partisanship, responsibility, and support for mental health treatment. Socius 6, Article 2378023120921652.

[10] Mark Nichter. 1981. Idioms of distress: Alternatives in the expression of psychosocial distress: A case study from South India. Culture, Medicine and Psychiatry 5, 4, 379-408.

[11] Sachin R. Pendse, Kate Niederhoffer, and Amit Sharma. 2019. Cross-cultural differences in the use of online mental health support forums. Proceedings of the ACM on Human-Computer Interaction 3, CSCW, Article 67, 29 pages. https://doi.org/10.1145/3359169

[12] Sachin R. Pendse, Neha Kumar, and Munmun De Choudhury. 2023. Marginalization and the construction of mental illness narratives online: foregrounding institutions in technology-mediated care. Proceedings of the ACM on Human-Computer Interaction 7, CSCW2, Article 300, 30 pages. https://doi.org/10.1145/3579593

[13] James W. Pennebaker, Ryan L. Boyd, Kayla Jordan, and Kate Blackburn. 2015. The development and psychometric properties of LIWC2015. Technical Report. University of Texas at Austin.

[14] Pew Research Center. 2024. Changing Partisan Coalitions in a Politically Divided Nation: Partisanship in Rural, Suburban, and Urban Communities. Technical Report. Pew Research Center, Washington, DC.

[15] Damon C. Roberts and Stephen M. Utych. 2020. Linking gender, language, and partisanship: Developing a database of masculine and feminine words. Political Research Quarterly 73, 1, 40-50.

[16] Philip Schwadel. 2017. The Republicanization of evangelical Protestants in the United States: An examination of the sources of political realignment. Social Science Research 62, 238-254.

The Role of Partisan Culture in Mental Health Language Online
Supplementary Material
Supplement E
Filtered Mental Health Language

**Prompt**

Please read in the following list of terms, and return the terms that are related to mental health. Please make sure that only terms from the inputted list are present in the outputted list (i.e. do not introduce any new terms that are not present in the original list). Please also return terms as a list in JSON format. Note: terms may be multiple words.

**Filtered Terms**

signs
intellectual
compulsive
problems
cognitive
self
physiological
stress
alzheimer
traumatic
ptsd
treatment
neurocognitive
psychiatric
relationship
disturbance
disturbances
bipolar
amnesia
sleep
mood
developmental
disorder
delusions
anxiety
hallucinations
diagnostic
disorders
insomnia
dysphoria
adhd
dissociative
suicidal
deficits
obsessive
trauma
psychotic
depression
persistent
medical
delirium
behaviors
manic
psychological
separation
diagnosis
illness
issues
impairment
depressive
behavioral
somatic
chronic
hypomanic
emotional
schizophrenia
neurological
dysfunction
remission
gambling
antisocial
fear
panic
mental
nervosa
medications
conditions
intoxication
health
apnea
condition
personality
comorbid
withdrawal
suicide
medication
symptom
abuse
generalized
symptoms
clinical
prognostic

The Role of Partisan Culture in Mental Health Language Online
Supplementary Material
Supplement F
Extended Analysis Tables

Below, we present the full tables of findings for each scope of our analysis (expressive differences, clinical differences, and polarization-related differences). This includes the top fifteen most distinct words for each set of compared populations, and differences in use of language tied to select psycholinguistic attributes from the Linguistic Inquiry and Word Count (LIWC) tool. Our specific rationale for use of these approaches can be found in Section 3 of the main text, with further motivation from literature for each chosen LIWC category in Supplement D. Each scope of analysis includes a comparison between matched Democrat and Republican users, matched Republican and Unaffiliated-R users, and matched Democrat and Unaffiliated-R users. Note that all linguistic comparisons were conducted using Welch's t-test. To account for multiple comparisons, we adjusted p-values using the False Discovery Rate method, with statistical significance set at $p < .05$.

## Partisan Expressive Differences

**Distinct Keywords, Reps and Dems**

| SAGE | Democrat | Republican | SAGE |
|---|---|---|---|
| 0.6638 | ADHD | local | 0.3421 |
| 0.3582 | diagnosis | inside | 0.3186 |
| 0.3294 | dose | loved | 0.3023 |
| 0.3102 | partner | please | 0.2610 |
| 0.2934 | brain | female | 0.2467 |
| 0.2824 | shitty | degree | 0.2242 |
| 0.2706 | psychiatrist | god | 0.2130 |
| 0.2549 | system | business | 0.2104 |
| 0.2482 | professional | dating | 0.2086 |
| 0.2430 | definitely | dad | 0.1945 |
| 0.2298 | super | date | 0.1920 |
| 0.2261 | autistic | jobs | 0.1891 |
| 0.2240 | diagnosed | college | 0.1846 |
| 0.2224 | tend | OCD | 0.1820 |
| 0.2221 | important | married | 0.1811 |

Table 1: Open vocabulary based key phrases, based on SAGE, Democrat and Republican users. Democrat users use language that mentions specific mental health disorders, professionals, or treatments. Republican users use language that alludes to social relationships, day-to-day life, and religion.

**Psycholinguistic Differences, Reps and Dems**

| Dimension | Democrat Mean | Republican Mean | Adj. p value |
|---|---|---|---|
| Social (R) | 12.32% $\pm$ 13.35% | 12.93% $\pm$ 13.80% | $1.30 \times 10^{-163}$ |
| Male (R) | 1.24% $\pm$ 4.66% | 1.38% $\pm$ 4.91% | $1.95 \times 10^{-64}$ |
| Female (R) | 1.24% $\pm$ 4.61% | 1.44% $\pm$ 4.92% | $6.37 \times 10^{-131}$ |
| Cognitive Processing (D) | 14.57% $\pm$ 13.52% | 14.26% $\pm$ 13.59% | $3.80 \times 10^{-44}$ |
| Positive Emotion | 5.76% $\pm$ 10.07% | 5.79% $\pm$ 10.47% | 0.131248 |
| Negative Emotion (D) | 5.41% $\pm$ 9.19% | 5.36% $\pm$ 9.19% | $3.46 \times 10^{-4}$ |
| Anxiety | 0.82% $\pm$ 3.22% | 0.82% $\pm$ 3.26% | 0.601142 |
| Anger (D) | 1.98% $\pm$ 5.95% | 1.91% $\pm$ 5.88% | $3.65 \times 10^{-12}$ |
| Feel (D) | 1.25% $\pm$ 4.05% | 1.24% $\pm$ 4.08% | 0.576841 |
| Bio (D) | 4.60% $\pm$ 8.56% | 4.52% $\pm$ 8.62% | $1.43 \times 10^{-8}$ |
| Body (D) | 1.23% $\pm$ 4.33% | 1.20% $\pm$ 4.32% | $4.82 \times 10^{-7}$ |
| Health | 1.88% $\pm$ 5.26% | 1.90% $\pm$ 5.38% | 0.0653815 |
| Affiliation (R) | 2.18% $\pm$ 5.91% | 2.33% $\pm$ 6.36% | $1.48 \times 10^{-50}$ |
| Work (R) | 3.03% $\pm$ 6.80% | 3.06% $\pm$ 7.02% | $4.21 \times 10^{-3}$ |
| Leisure (R) | 1.31% $\pm$ 4.78% | 1.35% $\pm$ 4.81% | $2.84 \times 10^{-5}$ |
| Home (R) | 0.44% $\pm$ 2.42% | 0.47% $\pm$ 2.53% | $2.55 \times 10^{-15}$ |
| Money (R) | 0.89% $\pm$ 3.72% | 0.95% $\pm$ 3.94% | $4.36 \times 10^{-25}$ |
| Religion (R) | 0.30% $\pm$ 2.57% | 0.35% $\pm$ 2.93% | $1.35 \times 10^{-29}$ |
| Death (R) | 0.26% $\pm$ 1.88% | 0.28% $\pm$ 2.02% | $2.95 \times 10^{-13}$ |

Table 2: Significant LIWC Dimensions, Expressive Differences, Democrat and Republican users. Democrat users use more language that suggests processing events that have happened. Republicans use language that suggests describing about day-to-day life events and social relationships. Means are formatted as mean $\pm$ standard deviation. All p-values were adjusted for the False Discovery Rate.

| Distinct Keywords, Reps and Unaff-R | | | |
|---|---|---|---|
| SAGE | Republican | Unaffiliated | SAGE |
| 0.6050 | business | BPD | 0.9080 |
| 0.5851 | local | ADHD | 0.6747 |
| 0.4359 | jobs | diagnosis | 0.5952 |
| 0.4209 | white | trauma | 0.5600 |
| 0.4194 | degree | partner | 0.5554 |
| 0.3677 | pay | dose | 0.5391 |
| 0.3647 | black | relate | 0.5180 |
| 0.3637 | buy | wanna | 0.5176 |
| 0.3630 | paying | psychiatrist | 0.5046 |
| 0.3623 | married | okay | 0.5014 |
| 0.3513 | gay | definitely | 0.4766 |
| 0.3455 | options | struggle | 0.4717 |
| 0.3109 | simply | hospital | 0.4685 |
| 0.3039 | perhaps | myself | 0.4672 |
| 0.2989 | police | cry | 0.4664 |

Table 3: Open vocabulary based key phrases, based on SAGE, Republican and Unaffiliated-R users. Republican users use language that alludes to identity, occupation and class, and places of particular cultural advocacy.

| Psycholinguistic Differences, Reps and Unaff-R | | | |
|---|---|---|---|
| Dimension | Republican Mean | Unaffiliated Mean | Adj. p value |
| Social (R) | 12.93% $\pm$ 13.80% | 11.85% $\pm$ 12.83% | $2.23 \times 10^{-308}$ |
| Male (R) | 1.38% $\pm$ 4.91% | 1.16% $\pm$ 4.48% | $1.03 \times 10^{-115}$ |
| Female (R) | 1.44% $\pm$ 4.92% | 1.13% $\pm$ 4.16% | $1.76 \times 10^{-259}$ |
| Cognitive Processing (U) | 14.26% $\pm$ 13.59% | 14.69% $\pm$ 13.23% | $4.73 \times 10^{-60}$ |
| Positive Emotion (U) | 5.79% $\pm$ 10.47% | 6.40% $\pm$ 10.81% | $0.001$ |
| Negative Emotion (R) | 5.36% $\pm$ 9.19% | 5.23% $\pm$ 8.67% | $1.77 \times 10^{-13}$ |
| Anxiety (U) | 0.82% $\pm$ 3.26% | 0.90% $\pm$ 3.15% | $7.92 \times 10^{-39}$ |
| Anger (R) | 1.91% $\pm$ 5.88% | 1.59% $\pm$ 5.13% | $1.45 \times 10^{-192}$ |
| Feel (U) | 1.24% $\pm$ 4.08% | 1.53% $\pm$ 4.29% | $2.47 \times 10^{-248}$ |
| Bio (R) | 4.52% $\pm$ 8.62% | 4.39% $\pm$ 7.94% | $3.18 \times 10^{-16}$ |
| Body (R) | 1.20% $\pm$ 4.32% | 1.04% $\pm$ 3.74% | $5.33 \times 10^{-85}$ |
| Health (U) | 1.90% $\pm$ 5.38% | 2.05% $\pm$ 5.20% | $5.12 \times 10^{-46}$ |
| Affiliation (U) | 2.33% $\pm$ 6.36% | 2.36% $\pm$ 6.13% | 0.021 |
| Work (R) | 3.06% $\pm$ 7.02% | 2.62% $\pm$ 6.14% | $1.15 \times 10^{-250}$ |
| Leisure (R) | 1.35% $\pm$ 4.81% | 1.28% $\pm$ 4.65% | $6.10 \times 10^{-12}$ |
| Home (R) | 0.47% $\pm$ 2.53% | 0.42% $\pm$ 2.25% | $3.80 \times 10^{-33}$ |
| Money (R) | 0.95% $\pm$ 3.94% | 0.65% $\pm$ 2.98% | $2.23 \times 10^{-308}$ |
| Religion (R) | 0.35% $\pm$ 2.93% | 0.25% $\pm$ 2.22% | $1.18 \times 10^{-88}$ |
| Death | 0.28% $\pm$ 2.02% | 0.27% $\pm$ 1.93% | 0.142 |

Table 4: Significant LIWC Dimensions, Expressive Differences, Republican and Unaffiliated-R users. Republican users have lower levels of language suggestive of processing their (health) experiences within online mental health forums, and higher levels of language suggestive of day-to-day issues. Means are formatted as mean $\pm$ standard deviation. All p-values were adjusted for the False Discovery Rate.

| Distinct Keywords, Dems and Unaff-D | | | |
|---|---|---|---|
| SAGE | Democrat | Unaffiliated | SAGE |
| 0.4808 | certainly | BPD | 0.9890 |
| 0.4789 | bullshit | wanna | 0.6503 |
| 0.4578 | paying | relate | 0.5888 |
| 0.4418 | white | cry | 0.5625 |
| 0.4333 | business | struggling | 0.5419 |
| 0.4185 | society | trauma | 0.4898 |
| 0.4007 | power | episode | 0.4778 |
| 0.3923 | black | suicidal | 0.4635 |
| 0.3890 | gay | anxious | 0.4630 |
| 0.3753 | plenty | myself | 0.4482 |
| 0.3711 | history | tired | 0.4423 |
| 0.3675 | line | haha | 0.4422 |
| 0.3618 | poor | panic | 0.4025 |
| 0.3597 | behavior | feel | 0.3914 |
| 0.3574 | women | felt | 0.3903 |

Table 5: Open vocabulary based key phrases, based on SAGE, Democrat and Unaffiliated-D users. Democrat users use language that hints at a socio-cultural and structural approach to mental health, in line with progressive perspectives.

| Psycholinguistic Differences, Dems and Unaff-D | | | |
|---|---|---|---|
| Dimension | Democrat Mean | Unaffiliated Mean | Adj. p value |
| Social (D) | 12.32% $\pm$ 13.35% | 11.59% $\pm$ 12.78% | $1.17 \times 10^{-156}$ |
| Male (D) | 1.24% $\pm$ 4.66% | 1.17% $\pm$ 4.50% | $5.05 \times 10^{-12}$ |
| Female (D) | 1.24% $\pm$ 4.61% | 1.15% $\pm$ 4.26% | $1.46 \times 10^{-22}$ |
| Cognitive Processing (U) | 14.57% $\pm$ 13.52% | 14.64% $\pm$ 13.20% | 0.016 |
| Positive Emotion (U) | 5.76% $\pm$ 10.07% | 6.33% $\pm$ 10.74% | $1.10 \times 10^{-146}$ |
| Negative Emotion (D) | 5.41% $\pm$ 9.19% | 5.15% $\pm$ 8.60% | $1.12 \times 10^{-45}$ |
| Anxiety (U) | 0.82% $\pm$ 3.22% | 0.89% $\pm$ 3.08% | $1.45 \times 10^{-22}$ |
| Anger (D) | 1.98% $\pm$ 5.95% | 1.63% $\pm$ 5.20% | $3.05 \times 10^{-206}$ |
| Feel (U) | 1.25% $\pm$ 4.05% | 1.53% $\pm$ 4.34% | $2.12 \times 10^{-217}$ |
| Bio (D) | 4.60% $\pm$ 8.56% | 4.34% $\pm$ 8.03% | $3.15 \times 10^{-52}$ |
| Body (D) | 1.23% $\pm$ 4.33% | 1.10% $\pm$ 3.97% | $2.81 \times 10^{-50}$ |
| Health | 1.88% $\pm$ 5.26% | 1.89% $\pm$ 5.04% | 0.328 |
| Affiliation (U) | 2.18% $\pm$ 5.91% | 2.30% $\pm$ 6.08% | $2.98 \times 10^{-23}$ |
| Work (D) | 3.03% $\pm$ 6.80% | 2.51% $\pm$ 6.03% | $2.23 \times 10^{-308}$ |
| Leisure (D) | 1.31% $\pm$ 4.78% | 1.28% $\pm$ 4.68% | $1.42 \times 10^{-3}$ |
| Home (D) | 0.44% $\pm$ 2.42% | 0.41% $\pm$ 2.20% | $4.75 \times 10^{-12}$ |
| Money (D) | 0.89% $\pm$ 3.72% | 0.64% $\pm$ 3.03% | $8.20 \times 10^{-281}$ |
| Religion (D) | 0.30% $\pm$ 2.57% | 0.25% $\pm$ 2.23% | $3.44 \times 10^{-24}$ |
| Death | 0.26% $\pm$ 1.88% | 0.26% $\pm$ 1.85% | 0.126 |

Table 6: Significant LIWC Dimensions, Expressive Differences, Democrat and Unaffiliated-D users. Democrat users use language indicative of conversations around day-to-day life and social relationships, and using health language to a roughly equal extent. Means are formatted as mean $\pm$ standard deviation. All p-values were adjusted for the False Discovery Rate.

## Partisan Differences in Clinical Language

| Distinct Keywords, Reps and Dems (Clinical) | | | |
|---|---|---|---|
| SAGE | Democrat | Republican | SAGE |
| 0.6218 | *ADHD* | hotline | 0.8799 |
| 0.3039 | partner | please | 0.6842 |
| 0.2988 | incredibly | loved | 0.6584 |
| 0.2788 | *diagnosis* | *schizophrenia* | 0.5886 |
| 0.2770 | dose | struggling | 0.5857 |
| 0.2686 | disability | god | 0.3313 |
| 0.2671 | function | watch | 0.2881 |
| 0.2620 | brain | OCD | 0.2757 |
| 0.2591 | psychiatrist | dating | 0.2631 |
| 0.2508 | manage | *suicide* | 0.2577 |
| 0.2481 | important | woman | 0.2541 |
| 0.2415 | definitely | date | 0.2522 |
| 0.2272 | professional | college | 0.2155 |
| 0.2194 | system | women | 0.2104 |
| 0.2164 | behavior | *PTSD* | 0.2081 |

Table 7: Open vocabulary based key phrases in posts with clinical words, based on SAGE, Democrat and Republican users. Words from our clinical lexicon are italicized. Republican users use language that suggests a familiarity with clinical diagnoses, but a reliance on non-medical sources of care. Democrat users use language that further emphasizes clinical and medical models of mental illness.

| Psycholinguistic Differences, Reps and Dems (Clinical) | | | |
|---|---|---|---|
| Dimension | Democrat Mean | Republican Mean | Adj. p value |
| Social (R) | 11.47% $\pm$ 8.99% | 11.84% $\pm$ 9.33% | $2.24 \times 10^{-22}$ |
| Male (R) | 0.89% $\pm$ 2.68% | 0.99% $\pm$ 2.81% | $5.07 \times 10^{-17}$ |
| Female (R) | 0.98% $\pm$ 3.05% | 1.15% $\pm$ 3.32% | $3.19 \times 10^{-39}$ |
| Cognitive Processing (D) | 16.49% $\pm$ 9.05% | 15.89% $\pm$ 8.96% | $3.30 \times 10^{-60}$ |
| Positive Emotion (D) | 4.85% $\pm$ 4.92% | 4.71% $\pm$ 4.89% | $7.60 \times 10^{-11}$ |
| Negative Emotion (R) | 7.00% $\pm$ 6.98% | 7.24% $\pm$ 7.09% | $8.80 \times 10^{-16}$ |
| Anxiety (R) | 1.78% $\pm$ 3.74% | 1.91% $\pm$ 4.01% | $3.41 \times 10^{-17}$ |
| Anger (R) | 1.63% $\pm$ 3.34% | 1.63% $\pm$ 3.33% | 0.943 |
| Feel | 1.39% $\pm$ 2.58% | 1.41% $\pm$ 2.61% | 0.050 |
| Bio | 6.19% $\pm$ 6.99% | 6.18% $\pm$ 7.08% | 0.829 |
| Body (R) | 1.36% $\pm$ 3.18% | 1.43% $\pm$ 3.33% | $1.17 \times 10^{-6}$ |
| Health (D) | 3.85% $\pm$ 5.82% | 3.77% $\pm$ 5.87% | $4.64 \times 10^{-4}$ |
| Affiliation (R) | 1.90% $\pm$ 3.26% | 1.95% $\pm$ 3.30% | $1.04 \times 10^{-3}$ |
| Work (D) | 3.30% $\pm$ 4.61% | 3.13% $\pm$ 4.55% | $2.08 \times 10^{-17}$ |
| Leisure (R) | 1.04% $\pm$ 2.51% | 1.07% $\pm$ 2.55% | $5.69 \times 10^{-3}$ |
| Home (R) | 0.40% $\pm$ 1.41% | 0.43% $\pm$ 1.48% | $5.79 \times 10^{-7}$ |
| Money | 0.65% $\pm$ 2.06% | 0.66% $\pm$ 2.11% | 0.158 |
| Religion (R) | 0.19% $\pm$ 1.07% | 0.22% $\pm$ 1.17% | $1.39 \times 10^{-10}$ |
| Death (R) | 0.41% $\pm$ 1.95% | 0.47% $\pm$ 2.02% | $1.20 \times 10^{-11}$ |

Table 8: Significant LIWC Dimensions, Clinical Differences, Democrat and Republican users. In clinical posts, we find higher use of biological language among Republican users, and higher use of health language from Democrat users, a shift from our analysis of all posts. This is suggestive of a more somatic framing of distress from Republican users. Means are formatted as mean $\pm$ standard deviation. All p-values were adjusted for the False Discovery Rate.

| Distinct Keywords, Reps and Unaff-R (Clinical) | | | |
|---|---|---|---|
| SAGE | Republican | Unaffiliated | SAGE |
| 0.4811 | god | BPD | 0.6600 |
| 0.4620 | married | struggling | 0.5821 |
| 0.4481 | anti | partner | 0.5537 |
| 0.4421 | men | *ADHD* | 0.4857 |
| 0.4178 | women | wanna | 0.4757 |
| 0.4159 | man | definitely | 0.4294 |
| 0.3679 | *psychotic* | okay | 0.4268 |
| 0.3606 | simply | crying | 0.4163 |
| 0.3526 | drug | cry | 0.4001 |
| 0.3426 | woman | deserve | 0.3873 |
| 0.3369 | blood | psychosis | 0.3834 |
| 0.3367 | quit | study | 0.3605 |
| 0.3273 | drugs | *diagnosis* | 0.3579 |
| 0.3241 | poor | relate | 0.3524 |
| 0.3214 | society | sorry | 0.3390 |

Table 9: Open vocabulary based key phrases in posts with clinical language, based on SAGE, Republican and Unaffiliated-R users. Words from our clinical lexicon are italicized. Republican partisan culture around religion influences expressions of distress—*god* is the most distinctly used word by Republican users.

| Psycholinguistic Differences, Reps and Unaff-R (Clinical) | | | |
|---|---|---|---|
| Dimension | Republican Mean | Unaffiliated Mean | Adj. p value |
| Social (R) | 11.96% $\pm$ 9.30% | 11.27% $\pm$ 8.68% | $1.39 \times 10^{-58}$ |
| Male (R) | 1.00% $\pm$ 2.82% | 0.91% $\pm$ 2.59% | $1.04 \times 10^{-13}$ |
| Female (R) | 1.16% $\pm$ 3.32% | 1.00% $\pm$ 2.96% | $3.34 \times 10^{-26}$ |
| Cognitive Processing (U) | 16.03% $\pm$ 8.89% | 16.53% $\pm$ 8.69% | $1.09 \times 10^{-32}$ |
| Positive Emotion (U) | 4.76% $\pm$ 4.92% | 4.95% $\pm$ 4.86% | $4.56 \times 10^{-16}$ |
| Negative Emotion (R) | 7.31% $\pm$ 7.09% | 6.98% $\pm$ 6.74% | $3.27 \times 10^{-24}$ |
| Anxiety (R) | 1.95% $\pm$ 4.06% | 1.86% $\pm$ 3.58% | $1.63 \times 10^{-6}$ |
| Anger (R) | 1.63% $\pm$ 3.30% | 1.47% $\pm$ 3.06% | $3.93 \times 10^{-29}$ |
| Feel (U) | 1.44% $\pm$ 2.62% | 1.68% $\pm$ 2.75% | $6.03 \times 10^{-83}$ |
| Bio (R) | 6.26% $\pm$ 7.11% | 6.01% $\pm$ 6.62% | $3.97 \times 10^{-14}$ |
| Body (R) | 1.45% $\pm$ 3.34% | 1.30% $\pm$ 3.02% | $3.33 \times 10^{-24}$ |
| Health | 3.82% $\pm$ 5.91% | 3.80% $\pm$ 5.57% | 0.319 |
| Affiliation | 1.96% $\pm$ 3.31% | 1.99% $\pm$ 3.19% | 0.082 |
| Work (R) | 3.16% $\pm$ 4.57% | 2.93% $\pm$ 4.22% | $4.15 \times 10^{-27}$ |
| Leisure (R) | 1.09% $\pm$ 2.55% | 1.03% $\pm$ 2.43% | $2.12 \times 10^{-6}$ |
| Home (R) | 0.43% $\pm$ 1.49% | 0.41% $\pm$ 1.36% | $1.16 \times 10^{-4}$ |
| Money (R) | 0.66% $\pm$ 2.12% | 0.51% $\pm$ 1.71% | $6.57 \times 10^{-68}$ |
| Religion (R) | 0.23% $\pm$ 1.19% | 0.18% $\pm$ 0.96% | $2.19 \times 10^{-24}$ |
| Death | 0.47% $\pm$ 2.01% | 0.46% $\pm$ 1.94% | 0.080 |

Table 10: Significant LIWC Dimensions, Clinical Differences, Republican and Unaffiliated-R users. Republican users have higher levels of language within their posts centered on social relationships and day to day life, similar to Democrat users. Means are formatted as mean $\pm$ standard deviation. All p-values were adjusted for the False Discovery Rate.

| Distinct Keywords, Dems and Unaff-D (Clinical) | | | |
|---|---|---|---|
| SAGE | Democrat | Unaffiliated | SAGE |
| 0.5907 | certainly | BPD | 0.8527 |
| 0.4439 | *condition* | cry | 0.6145 |
| 0.4433 | number | crying | 0.5220 |
| 0.4296 | power | struggling | 0.4683 |
| 0.4250 | drug | episode | 0.4583 |
| 0.4238 | society | relate | 0.4450 |
| 0.4128 | disability | kinda | 0.4031 |
| 0.3970 | *conditions* | tired | 0.3942 |
| 0.3953 | behavior | episodes | 0.3937 |
| 0.3931 | spectrum | myself | 0.3889 |
| 0.3851 | line | sad | 0.3593 |
| 0.3397 | exercise | *schizophrenia* | 0.3569 |
| 0.3384 | men | feel | 0.3438 |
| 0.3209 | ability | *trauma* | 0.3424 |
| 0.2982 | women | horrible | 0.3385 |

Table 11: Open vocabulary based key phrases from clinical posts, based on SAGE, Democrat and Unaffiliated-D users. Words from our clinical lexicon are italicized. Democrat users utilize language suggestive of progressive movements that understand mental illness to be a chronic condition.

| Psycholinguistic Differences, Dems and Unaff-D (Clinical) | | | |
|---|---|---|---|
| Dimension | Democrat Mean | Unaffiliated Mean | Adj. p value |
| Social (D) | 11.47% $\pm$ 8.98% | 10.98% $\pm$ 8.55% | $6.23 \times 10^{-31}$ |
| Male | 0.89% $\pm$ 2.68% | 0.87% $\pm$ 2.52% | 0.130 |
| Female | 0.98% $\pm$ 3.04% | 1.00% $\pm$ 2.99% | 0.116 |
| Cognitive Processing | 16.52% $\pm$ 9.04% | 16.47% $\pm$ 8.52% | 0.292 |
| Positive Emotion | 4.84% $\pm$ 4.90% | 4.84% $\pm$ 4.77% | 0.769 |
| Negative Emotion | 6.98% $\pm$ 6.96% | 6.97% $\pm$ 6.55% | 0.769 |
| Anxiety (U) | 1.77% $\pm$ 3.73% | 1.84% $\pm$ 3.48% | $2.76 \times 10^{-5}$ |
| Anger (D) | 1.62% $\pm$ 3.31% | 1.53% $\pm$ 3.00% | $2.70 \times 10^{-10}$ |
| Feel (U) | 1.39% $\pm$ 2.57% | 1.65% $\pm$ 2.61% | $9.87 \times 10^{-92}$ |
| Bio (D) | 6.20% $\pm$ 6.98% | 5.89% $\pm$ 6.56% | $3.04 \times 10^{-20}$ |
| Body (D) | 1.36% $\pm$ 3.17% | 1.32% $\pm$ 3.09% | 0.014 |
| Health (D) | 3.86% $\pm$ 5.82% | 3.66% $\pm$ 5.41% | $7.36 \times 10^{-14}$ |
| Affiliation | 1.90% $\pm$ 3.26% | 1.93% $\pm$ 3.14% | 0.080 |
| Work (D) | 3.30% $\pm$ 4.61% | 2.84% $\pm$ 4.09% | $4.60 \times 10^{-108}$ |
| Leisure (D) | 1.04% $\pm$ 2.50% | 1.00% $\pm$ 2.39% | 0.002 |
| Home | 0.39% $\pm$ 1.40% | 0.40% $\pm$ 1.34% | 0.351 |
| Money (D) | 0.64% $\pm$ 2.05% | 0.51% $\pm$ 1.68% | $1.15 \times 10^{-46}$ |
| Religion (D) | 0.19% $\pm$ 1.05% | 0.17% $\pm$ 0.97% | $3.53 \times 10^{-5}$ |
| Death (U) | 0.41% $\pm$ 1.95% | 0.43% $\pm$ 1.85% | 0.040 |

Table 12: Significant LIWC Dimensions, Clinical Differences, Democrat and Unaffiliated-D users. Democrat users have higher levels of language within their posts centered on social relationships and day to day life. Means are formatted as mean $\pm$ standard deviation. All p-values were adjusted for the False Discovery Rate.

## Partisan Differences in Polarization Language

| Distinct Keywords, Reps and Dems (Polarization) | | | |
|---|---|---|---|
| SAGE | Democrat | Republican | SAGE |
| 0.6598 | ADHD | ugly | 0.3216 |
| 0.3523 | diagnosis | degree | 0.2359 |
| 0.3036 | brain | dad | 0.2333 |
| 0.3015 | psychiatrist | watch | 0.2222 |
| 0.2873 | partner | god | 0.2196 |
| 0.2785 | shitty | date | 0.2107 |
| 0.2329 | professional | heart | 0.2091 |
| 0.2189 | certainly | OCD | 0.2085 |
| 0.2149 | important | college | 0.2015 |
| 0.2047 | system | dating | 0.2014 |
| 0.2007 | diagnosed | married | 0.1970 |
| 0.1996 | definitely | classes | 0.1967 |
| 0.1992 | trump | baby | 0.1952 |
| 0.1982 | ADD | *gun* | 0.1928 |
| 0.1981 | specific | son | 0.1818 |

Table 13: Open vocabulary based key phrases in posts with polarization words, based on SAGE, Democrat and Republican users. Words from the polarization language lexicon are italicized. Partisan political rhetoric does appear in expressions of distress from both Democrat and Republican users.

| Psycholinguistic Differences, Reps and Dems (Polarization) | | | |
|---|---|---|---|
| Dimension | Democrat Mean | Republican Mean | Adj. p value |
| Social (R) | 14.92% ± 11.01% | 15.43% ± 11.29% | $1.10 \times 10^{-59}$ |
| Male (R) | 1.22% ± 3.41% | 1.34% ± 3.55% | $1.10 \times 10^{-34}$ |
| Female (R) | 1.36% ± 3.94% | 1.57% ± 4.23% | $3.68 \times 10^{-75}$ |
| Cognitive Processing (D) | 15.84% ± 10.03% | 15.60% ± 9.99% | $6.53 \times 10^{-18}$ |
| Positive Emotion (D) | 5.15% ± 5.82% | 5.10% ± 5.88% | $9.83 \times 10^{-4}$ |
| Negative Emotion | 7.76% ± 9.02% | 7.79% ± 9.02% | 0.212 |
| Anxiety (R) | 0.99% ± 2.64% | 1.02% ± 2.71% | $1.77 \times 10^{-4}$ |
| Anger (D) | 3.53% ± 7.17% | 3.48% ± 7.11% | $5.26 \times 10^{-3}$ |
| Feel (R) | 1.32% ± 2.85% | 1.34% ± 2.94% | $2.07 \times 10^{-3}$ |
| Bio (D) | 5.20% ± 7.32% | 5.05% ± 7.18% | $2.70 \times 10^{-13}$ |
| Body (D) | 1.52% ± 3.93% | 1.48% ± 3.85% | $1.85 \times 10^{-4}$ |
| Health | 1.85% ± 3.56% | 1.85% ± 3.56% | 0.850 |
| Affiliation (R) | 2.20% ± 3.90% | 2.29% ± 4.02% | $2.63 \times 10^{-14}$ |
| Work | 2.97% ± 4.85% | 2.96% ± 4.90% | 0.601 |
| Leisure (R) | 1.13% ± 2.89% | 1.18% ± 2.98% | $2.94 \times 10^{-10}$ |
| Home (R) | 0.42% ± 1.65% | 0.45% ± 1.71% | $1.40 \times 10^{-7}$ |
| Money (R) | 0.85% ± 2.70% | 0.89% ± 2.72% | $4.51 \times 10^{-5}$ |
| Religion (R) | 0.32% ± 1.84% | 0.35% ± 1.91% | $7.67 \times 10^{-10}$ |
| Death (R) | 0.39% ± 1.94% | 0.43% ± 2.09% | $9.07 \times 10^{-13}$ |

Table 14: Significant LIWC Dimensions, Polarization Differences, Democrat and Republican users. We find similar patterns to our expressive and clinical analyses, with more cognitive processing language from Democrat users, and language indicative of social relationships and day-to-day life from Republican users. Means are formatted as mean ± standard deviation. All p-values were adjusted for the False Discovery Rate.

| Distinct Keywords, Reps and Unaff-R (Polarization) | | | |
|---|---|---|---|
| SAGE | Republican | Unaffiliated | SAGE |
| 0.8192 | *gun* | BPD | 0.8995 |
| 0.5704 | business | struggling | 0.7006 |
| 0.5016 | white | ADHD | 0.6650 |
| 0.5016 | black | diagnosis | 0.5825 |
| 0.4774 | jobs | partner | 0.5147 |
| 0.4365 | married | psychiatrist | 0.5045 |
| 0.4092 | *rape* | wanna | 0.5006 |
| 0.4064 | gay | trauma | 0.4855 |
| 0.4054 | degree | relate | 0.4607 |
| 0.4046 | buy | cry | 0.4523 |
| 0.3703 | police | crying | 0.4305 |
| 0.3639 | ass | suicidal | 0.4238 |
| 0.3626 | perhaps | myself | 0.4206 |
| 0.3617 | pay | okay | 0.4194 |
| 0.3503 | paying | recently | 0.3912 |

Table 15: Open vocabulary based key phrases in posts with polarization language, based on SAGE, Republican and Unaffiliated-R. Words from the polarization language lexicon are italicized. Partisan cultural positions and debates about identity are reflected in words used by Republican users.

| Psycholinguistic Differences, Reps and Unaff-R (Polarization) | | | |
|---|---|---|---|
| Dimension | Republican Mean | Unaffiliated Mean | Adj. p value |
| Social (R) | 15.44% ± 11.28% | 14.43% ± 10.45% | $3.82 \times 10^{-170}$ |
| Male (R) | 1.34% ± 3.54% | 1.19% ± 3.21% | $8.52 \times 10^{-44}$ |
| Female (R) | 1.57% ± 4.22% | 1.32% ± 3.68% | $1.86 \times 10^{-83}$ |
| Cognitive Processing (U) | 15.61% ± 9.99% | 16.34% ± 9.63% | $1.84 \times 10^{-108}$ |
| Positive Emotion (U) | 5.11% ± 5.88% | 5.36% ± 5.73% | $1.09 \times 10^{-39}$ |
| Negative Emotion (R) | 7.77% ± 8.98% | 7.45% ± 8.30% | $9.92 \times 10^{-29}$ |
| Anxiety (R) | 1.02% ± 2.71% | 1.15% ± 2.59% | $1.17 \times 10^{-43}$ |
| Anger (R) | 3.46% ± 7.05% | 2.88% ± 6.23% | $3.04 \times 10^{-150}$ |
| Feel (U) | 1.34% ± 2.90% | 1.66% ± 3.01% | $2.90 \times 10^{-232}$ |
| Bio (R) | 5.04% ± 7.15% | 4.81% ± 6.57% | $2.26 \times 10^{-23}$ |
| Body (R) | 1.47% ± 3.83% | 1.28% ± 3.36% | $5.96 \times 10^{-61}$ |
| Health (U) | 1.85% ± 3.56% | 2.03% ± 3.58% | $1.45 \times 10^{-52}$ |
| Affiliation (U) | 2.29% ± 4.02% | 2.34% ± 3.85% | $2.15 \times 10^{-4}$ |
| Work (R) | 2.97% ± 4.90% | 2.56% ± 4.24% | $7.38 \times 10^{-161}$ |
| Leisure (R) | 1.18% ± 2.98% | 1.10% ± 2.76% | $6.44 \times 10^{-17}$ |
| Home (R) | 0.45% ± 1.71% | 0.41% ± 1.49% | $2.82 \times 10^{-12}$ |
| Money (R) | 0.89% ± 2.73% | 0.64% ± 2.14% | $3.53 \times 10^{-217}$ |
| Religion (R) | 0.35% ± 1.90% | 0.26% ± 1.52% | $1.40 \times 10^{-58}$ |
| Death (R) | 0.43% ± 2.09% | 0.42% ± 1.91% | 0.013 |

Table 16: Significant LIWC Dimensions, Polarization Differences, Republican and Unaffiliated-R users. Posts from Republican users use significantly less affiliation language than unaffiliated users. Means are formatted as mean ± standard deviation. All p-values were adjusted for the False Discovery Rate.

| Distinct Keywords, Dems and Unaff-D (Polarization) | | | |
|---|---|---|---|
| SAGE | Democrat | Unaffiliated | SAGE |
| 1.475 | trump | BPD | 0.9829 |
| 0.4874 | certainly | wanna | 0.6161 |
| 0.4808 | *bullshit* | cry | 0.5959 |
| 0.4764 | white | struggling | 0.5690 |
| 0.4545 | power | relate | 0.5568 |
| 0.4382 | business | trauma | 0.5481 |
| 0.4356 | black | anxious | 0.5125 |
| 0.4309 | society | suicidal | 0.4753 |
| 0.4154 | insurance | myself | 0.4730 |
| 0.4026 | plenty | tired | 0.4496 |
| 0.3973 | line | mood | 0.4403 |
| 0.3823 | number | recently | 0.4402 |
| 0.3696 | behavior | panic | 0.4346 |
| 0.3665 | gay | felt | 0.4186 |
| 0.3665 | police | feel | 0.4057 |

Table 17: Open vocabulary based key phrases from polarization posts, based on SAGE, Democrat and Unaffiliated-D users. Words from the polarization lexicon are italicized. We observe aspects of structural and economic approaches to mental health reflected in language used distinctly from Democrat users.

| Psycholinguistic Differences, Dems and Unaff-D (Polarization) | | | |
|---|---|---|---|
| Dimension | Democrat Mean | Unaffiliated Mean | Adj. p value |
| Social (D) | 14.92% $\pm$ 11.00% | 14.16% $\pm$ 10.46% | $7.62 \times 10^{-92}$ |
| Male (D) | 1.22% $\pm$ 3.40% | 1.18% $\pm$ 3.21% | $5.40 \times 10^{-4}$ |
| Female | 1.36% $\pm$ 3.93% | 1.36% $\pm$ 3.78% | 0.881 |
| Cognitive Processing (U) | 15.86% $\pm$ 10.03% | 16.40% $\pm$ 9.59% | $6.84 \times 10^{-57}$ |
| Positive Emotion (U) | 5.15% $\pm$ 5.81% | 5.30% $\pm$ 5.70% | $3.09 \times 10^{-14}$ |
| Negative Emotion (D) | 7.74% $\pm$ 9.00% | 7.40% $\pm$ 8.12% | $1.39 \times 10^{-29}$ |
| Anxiety (U) | 0.99% $\pm$ 2.63% | 1.15% $\pm$ 2.56% | $1.41 \times 10^{-67}$ |
| Anger (D) | 3.52% $\pm$ 7.14% | 2.94% $\pm$ 6.27% | $1.63 \times 10^{-141}$ |
| Feel (U) | 1.32% $\pm$ 2.85% | 1.68% $\pm$ 3.06% | $3.60 \times 10^{-261}$ |
| Bio (D) | 5.19% $\pm$ 7.29% | 4.84% $\pm$ 6.61% | $4.21 \times 10^{-48}$ |
| Body (D) | 1.51% $\pm$ 3.91% | 1.36% $\pm$ 3.61% | $4.00 \times 10^{-33}$ |
| Health (U) | 1.85% $\pm$ 3.56% | 1.95% $\pm$ 3.44% | $8.09 \times 10^{-15}$ |
| Affiliation (U) | 2.21% $\pm$ 3.90% | 2.29% $\pm$ 3.81% | $1.86 \times 10^{-10}$ |
| Work (D) | 2.98% $\pm$ 4.85% | 2.51% $\pm$ 4.20% | $2.74 \times 10^{-195}$ |
| Leisure (D) | 1.13% $\pm$ 2.89% | 1.10% $\pm$ 2.72% | $2.38 \times 10^{-3}$ |
| Home | 0.43% $\pm$ 1.65% | 0.42% $\pm$ 1.52% | 0.179 |
| Money (D) | 0.85% $\pm$ 2.70% | 0.63% $\pm$ 2.12% | $4.80 \times 10^{-174}$ |
| Religion (D) | 0.32% $\pm$ 1.84% | 0.26% $\pm$ 1.55% | $1.45 \times 10^{-25}$ |
| Death | 0.39% $\pm$ 1.94% | 0.40% $\pm$ 1.86% | 0.175 |

Table 18: Significant LIWC Dimensions, Polarization Differences, Democrat and Unaffiliated-D users. Similar to Republican users, posts from Democrat users use less affiliation language than unaffiliated users. Means are formatted as mean $\pm$ standard deviation. All p-values were adjusted for the False Discovery Rate.

The Role of Partisan Culture in Mental Health Language Online
Supplementary Material
Supplement G
Temporal Change Analysis

**Republican and Democrat Users**

*Pre-2016*

In our dataset, there were 104,047 posts from Republican users before 2016, and 109,651 posts from Democrat users before 2016. Prior to 2016, we observe that Democrat users utilized more clinical language and with greater frequency, with Democrat users utilizing clinical language in 19.34% (standard deviation = 39.50%) of posts and 1.20% (standard deviation = 3.92%) of a given post on average, and Republican users utilizing clinical language in 17.97% (standard deviation = 38.40%) of posts and in 1.13% (standard deviation = 3.97%) of a given post on average (5.29 x 10^-16 and p < 7.65 x 10^-5, respectively, for the incidence and percentage of post comparisons)).

Looking to polarization language, prior to 2016, we observe that Democrat users also utilized more polarization language and with greater frequency, with Democrat users utilizing polarization language in 39.92% (standard deviation = 48.97%) of posts and 3.23% (standard deviation = 7.14%) of a given post on average, and Republican users utilizing polarization language in 37.82% (standard deviation = 48.49%) of posts and in 3.00% (standard deviation = 6.90%) of a given post on average (2.04 x 10^-23 and p < 1.12 x 10^-13, respectively, for the incidence and percentage of post comparisons).

*2016 and after*

In our dataset, there were 654,107 posts from Republican users in 2016 and after, and 609,219 posts from Democrat users in 2016 and after. Post-2016, we observe that Democrat users utilized more clinical language and with greater frequency, with Democrat users utilizing clinical language in 17.46% (standard deviation = 37.96%) of posts and 1.25% (standard deviation = 4.51%) of a given post on average, and Republican users utilizing clinical language in 16.18% (standard deviation = 36.83%) of posts and in 1.11% (standard deviation = 4.11%) of a given post on average (8.83 x 10^-83 and p < 1.17 x 10^-73, respectively, for the incidence and percentage of post comparisons).

Post-2016, we observe that Democrat users also utilized more polarization language and with greater frequency, with Democrat users utilizing polarization language in 36.59% (standard deviation = 48.17%) of posts and 3.22% (standard deviation = 7.50%) of a given post on average, and Republican users utilizing polarization language in 35.26% (standard deviation = 47.78%) of posts and in 3.10% (standard deviation = 7.34%) of a given post on average (9.29 x 10^-55 and p < 5.10 x 10^-20, respectively, for the incidence and percentage of post comparisons).

**Republican and Unaffiliated Users**

*Pre-2016*

In our dataset, there were 104,047 posts from Republican users before 2016, and 25,376 posts from matched unaffiliated users before 2016. Prior to 2016, we observe that unaffiliated users utilized more

clinical language and with greater frequency, with unaffiliated users utilizing clinical language in 23.31% (standard deviation = 42.28%) of posts and 1.36% (standard deviation = 4.21%) of a given post on average, and Republican users utilizing clinical language in 17.97% (standard deviation = 38.40%) of posts and in 1.13% (standard deviation = 3.97%) of a given post on average (3.08 x 10^-84 and p < 2.45 x 10^-16, respectively).

Looking to polarization language, we also observe that unaffiliated users also utilized more polarization language and with greater frequency, with unaffiliated users utilizing polarization language in 40.67% (standard deviation = 49.12%) of posts and 2.80% (standard deviation = 5.94%) of a given post on average, and Republican users utilizing polarization language in 37.82% (standard deviation = 48.49%) of posts and in 3.00% (standard deviation = 6.90%) of a given post on average (5.29 x 10^-17 and p < 1.41 x 10^-5, respectively).

*2016 and after*
In our dataset, there were 654,107 posts from Republican users in 2016 and after, and 347,813 posts from matched unaffiliated users in 2016 and after. We observe that unaffiliated users utilized more clinical language and with greater frequency, with unaffiliated users utilizing clinical language in 20.18% (standard deviation = 40.13%) of posts and 1.31% (standard deviation = 4.39%) of a given post on average, and Republican users utilizing clinical language in 16.18% (standard deviation = 36.83%) of posts and in 1.11% (standard deviation = 4.11%) of a given post on average (p < 2.23 x 10^-308 and p < 1.53 x 10^-120, respectively).

Looking to polarization language, we observe that Republican users utilized more polarization language and with greater frequency during and after 2016, with Republican users utilizing polarization language in 35.26% (standard deviation = 47.78%) of posts and 3.10% (standard deviation = 7.34%) of a given post on average, and unaffiliated users utilizing polarization language in 34.99% (standard deviation = 47.70%) of posts and in 2.66% (standard deviation = 6.56%) of a given post on average (p = 0.009 and 2.70 x 10^-191, respectively). **Note that this is the only shift we observe, among Republican users utilizing more polarization language after 2016.**

<u>**Democrat and Unaffiliated Users**</u>
*Pre-2016*
In our dataset, there were 109,651 posts from Democrat users before 2016, and 25,902 posts from matched unaffiliated users before 2016. Prior to 2016, we observe that unaffiliated users utilized more clinical language and with greater frequency, with unaffiliated users utilizing clinical language in 22.85% (standard deviation = 41.99%) of posts and 1.39% (standard deviation = 4.24%) of a given post on average, and Democrat users utilizing clinical language in 19.34% (standard deviation = 39.50%) of posts and in 1.20% (standard deviation = 3.92%) of a given post on average (5.43 x 10^-37 and p < 5.49 x 10^-12, respectively).

Looking to polarization language, we observe that Democrat users utilized more polarization language and with greater frequency during and after 2016, with Democrat users utilizing polarization language in

39.92% (standard deviation = 48.97%) of posts and 3.23% (standard deviation = 7.14%) of a given post on average, and unaffiliated users utilizing polarization language in 38.74% (standard deviation = 48.72%) of posts and in 2.77% (standard deviation = 6.30%) of a given post on average ($p = 0.0005$ and $3.04 \times 10^{-21}$, respectively).

*2016 and after*

In our dataset, there were 609,219 posts from Democrat users during and after 2016, and 308,241 posts from matched unaffiliated users after 2016. In 2016 and after, we observe that unaffiliated users utilized more clinical language and with greater frequency, with unaffiliated users utilizing clinical language in 20.35% (standard deviation = 40.26%) of posts and 1.32% (standard deviation = 4.38%) of a given post on average, and Democrat users utilizing clinical language in 17.46% (standard deviation = 37.96%) of posts and in 1.25% (standard deviation = 4.51%) of a given post on average ($2.84 \times 10^{-249}$ and $p < 8.86 \times 10^{-13}$, respectively).

Looking to polarization language, we observe that Democrat users utilized more polarization language and with greater frequency during and after 2016, with Democrat users utilizing polarization language in 36.59% (standard deviation = 48.17%) of posts and 3.22% (standard deviation = 7.50%) of a given post on average, and unaffiliated users utilizing polarization language in 35.38% (standard deviation = 47.81%) of posts and in 2.68% (standard deviation = 6.60%) of a given post on average ($4.32 \times 10^{-30}$ and $p < 2.10 \times 10^{-253}$, respectively).
